# Supplementary material for: Model selection of chaotic systems from data with hidden variables using sparse data assimilation
Source: arXiv:2105.10068 source file (2021-07-19)
Supplement: Supplementary file 1 [file main_SI.tex]

% \documentclass[12pt,letterpaper]{article}
% \usepackage[utf8]{inputenc}
% %\usepackage[catalan]{babel}
% \usepackage[english]{babel}
% \usepackage{amsfonts}
% \usepackage{amssymb}
% \usepackage[pdftex]{graphicx}
% \usepackage[font=small,labelfont=bf]{caption}
% \usepackage{epstopdf}
% \usepackage[T1]{fontenc}
% \usepackage{etoolbox}
% \usepackage{cleveref}
% \usepackage{multirow}
% \usepackage[top=1.4in, bottom=1.4in, left=0.8in, right=0.8in]{geometry}
% %\usepackage{lineno}
% %\linenumbers
% \usepackage{tikz}
% \usetikzlibrary{patterns}
% \usepackage{xcolor}
% \usepackage{subcaption}
% \usepackage{tikz-3dplot}
% \usepackage{array}
% \usepackage{rotating}
% \usepackage{ctable}
% \usepackage{geometry}
% \usepackage{color,soul}
% \usepackage{float}
% \usepackage{wrapfig}
% %\usepackage{hyperref}
% %\usepackage{cleveref}
% %\usepackage{autonum}
% \usepackage{algorithm}
% \usepackage[noend]{algpseudocode}
% \usepackage{listings}
% \usepackage{comment}
% \usepackage{mathtools}
% \usepackage{tabularx}
% % \usepackage[options]{algorithm2e,setspace}
% \usepackage{url}
% \usepackage{enumitem}
% \usepackage{longtable}

% \usepackage{algorithm}
% %\usepackage[algo2e]{algorithm2e} 
% % \usepackage{arevmath}     % For math symbols
% \usepackage[noend]{algpseudocode}
% \usepackage{amsmath}

% \usepackage{color, colortbl}
% \definecolor{name}{system}{definition}
% \definecolor{mygreen}{RGB}{28,172,0} % color values Red, Green, Blue
% \definecolor{mylilas}{RGB}{170,55,241}
% \definecolor{YellowHighlight}{rgb}{1,0.929,0.525}
% \definecolor{RedHighlight}{rgb}{0.9412,0.502,0.502}
% \definecolor{GreenHighlight}{rgb}{0.5961,0.9843,0.5961}

% \newcolumntype{M}[1]{>{\arraybackslash}m{#1}}
% \newcolumntype{N}{@{}m{0pt}@{}}

% \newcommand{\mathcolorbox}[2]{\colorbox{#1}{$\displaystyle #2$}}

% \newcommand{\mathbfgl}[1]{\boldsymbol{\mathbf{#1}}}

% \renewcommand{\baselinestretch}{1.3} 

% \allowdisplaybreaks

% \makeatletter
% \def\BState{\State\hskip-\ALG@thistlm}
% \makeatother

% \usetikzlibrary{arrows.meta}

% \usepackage{calc}

% \begin{document}

% \newlength\Dwidth
% \settowidth{\Dwidth}{\textbf{Sensors/Ladders}}
% \newcolumntype{C}{>{\centering}p{(\Dwidth-4\tabcolsep)/3}}

% \lstset{language=Matlab,%
%     %basicstyle=\color{red},
%     breaklines=true,%
%     morekeywords={matlab2tikz},
%     keywordstyle=\color{blue},%
%     morekeywords=[2]{1}, keywordstyle=[2]{\color{black}},
%     identifierstyle=\color{black},%
% %    stringstyle=\color{mylilas},
% %    commentstyle=\color{mygreen},%
%     showstringspaces=false,%without this there will be a symbol in the places where there is a space
%     numbers=left,%
%     numberstyle={\tiny \color{black}},% size of the numbers
%     numbersep=9pt, % this defines how far the numbers are from the text
% %    emph=[1]{for,end,break},emphstyle=[1]\color{red}, %some words to emphasise
%     %emph=[2]{word1,word2}, emphstyle=[2]{style},    
%     basicstyle=\linespread{0.9}\small\ttfamily,
% }

% \newcommand{\ipnp}{\ensuremath{_{i+1}^{n+1}}}
% \newcommand{\imnp}{\ensuremath{_{i-1}^{n+1}}}
% \newcommand{\inp}{\ensuremath{_{i}^{n+1}}}

% \newcommand{\ipn}{\ensuremath{_{i+1}^{n}}}
% \newcommand{\imn}{\ensuremath{_{i-1}^{n}}}
% \newcommand{\inn}{\ensuremath{_{i}^{n}}}

% \newcommand{\np}{\ensuremath{^{n+1}}}
% \newcommand{\n}{\ensuremath{^{n}}}

% \newcommand{\erf}{\ensuremath{\text{erf}}}

% \newcommand{\etaltri}{\emph{et al.}$\;$} 

% \newcommand{\red}{\textcolor{red}}
% \newcommand{\blue}{\textcolor{blue}}

% \newcommand{\ud}{\mathop{}\!\mathrm{d}}

% \title{Supplementary Information}

% %\author{H. Ribera, S. Shirman, A. V. Nguyen, N. M. Mangan}

% %\date{\today}

% %%%%%%%%%%%%%%%%%%%%%%%%%%%%%%%%%%%%%%%%%%%%%%%%%%%%%%%%%%%%%%%%%%%%%%     

% \maketitle

% %%%%%%%%%%%%%%%%%%%%%%%%%%%%%%%%%%%%%%%%%%%%%%%%%%%%%%%%%%%%%%%%%%%%%

% \vspace{1mm} 
% \tableofcontents
% \vspace{1mm} 

% \clearpage

% %%%%%%%%%%%%%%%%%%%%%%%%%%%%%%%%%%%%%%%%%%%%%%%%%%%%%%%%%%%%%%%%%%%%%

% \section*{Table of notation}
% \begin{center}
% \begin{longtable}{{p{3cm}p{6cm}p{5cm}}}
% %\caption{Notation table}\\
% \hline
% Variable name & Definition & Expression\\
% \specialrule{1.3pt}{1pt}{1pt}
% \endfirsthead
% \multicolumn{3}{l}%
% {\textit{Continued from previous page}} \\
% \hline
% Variable name & Definition & Expression\\
% \specialrule{1.3pt}{1pt}{1pt}
% \endhead
% \hline \multicolumn{3}{r}{\textit{Continued on next page}} \\
% \endfoot
% \hline
% \endlastfoot
%         $\mathbf{X}$ & State variable vector & \\
%         $\mathbf{Y}$ & Measurements vector & \\
%         $\mathbf{h}$ & Measurement function & $\mathbf{h}(\mathbf{X}) = \mathbf{Y} = \mathbf{X} + \mathcal{N}(0,\omega)$ \\
%         $\mathbf{p}$ & Parameter vector & \\
%         $R_f$ & Model enforcement term & $R_f = R_{f,0} \alpha^{\beta}$ \\
%         $R_{f,0}$ & Initial model enforcement & \\
%         $\alpha$ & \multirow{2}{*}{Model enforcement knobs} & \\
%         $\beta$ & & \\
%         $\beta_{\max}$ &  Maximum value for $\beta$ & \\
%         $A$ & Action & $A_E + R_f A_M + \lambda \Vert\mathbf{p}\Vert_1$ \\
%         $\hat{A}$ & Action & $A_E + R_f A_M$\\
%         $\omega$ & Standard deviation for noise & \\
%         $N$ & Number of time points & \\
%         $\Delta t$ & Time step & \\
%         $N_I$ & Number of initialisations & \\
%         $\mathbfgl{\Theta}$ & Library of functions & \\
%         $D$ & Dimension of the state variables & \\
%         $L$ & Dimension of the measurements & \\
%         $\hat{F_k}$ & Generic function for governing equation & $\sum_{j=1}^q p_{k,j} \theta_j$ \\
%         $F_k$ & Found governing equation & \\
%         $\mathbf{\hat{F}}$ & & $(\hat{F}_1,\hat{F}_2,\dots,\hat{F}_D)$\\
%         $\mathbf{F}$ & & $(F_1,F_2,\dots,F_D)$\\
%         $\mathbf{f}$ & discrete time dynamics model & \\
%         $\lambda$ & Sparsity knob & \\
%         $P$ & Total number of unknown parameters & $P=Dq$ \\
%         $p_{k,j}$ & Parameter of the $k$-th $\hat{F}$ with the $j$-th function in $\mathbfgl{\Theta}$ & \\
%         $\mathbf{X}^{\text{ini}}$ & Initialisation of $\mathbf{X}$ for VA & \\
%         $\mathbf{p}^{\text{ini}}$ & Initialisation of $\mathbf{p}$ for VA & \\
%         $\mathbf{X}^{\text{fin}}$ & Final solution of $\mathbf{X}$ found via VA & \\
%         $\mathbf{p}^{\text{fin}}$ & Final solution of $\mathbf{p}$ found via VA & \\        
%         $\mathbf{X}^{(\beta)}$ & Solution of $\mathbf{X}$ at the $\beta$-th step of VA & \\
%         $\mathbf{p}^{(\beta)}$ & Solution of $\mathbf{p}$ at the $\beta$-th step of VA & \\
%         $A_E$ & Measurement error & $\frac{1}{N}\sum_{i=1}^N \Vert \mathbf{X}(t_{i}) - \mathbf{Y}(t_{i}) \Vert^2$ \\
%         $A_M$ & Model error & $\frac{1}{N}\sum_{i=1}^{N-1} \left\{ \Vert \mathbf{X}(t_{i+1}) - \mathbf{f}(\mathbf{X}(t_i),\mathbf{p},\mathbf{\hat{F}}) \Vert^2 \right\}$ \\
%         $x_e$ & x measurement in the circuit & \\
%         $z_e$ & z measurement in the circuit & \\
%         $i$ & Index to sum over time points & \\
%         $j$ & Index to denote the $j$-th component of $\mathbfgl{\Theta}$ & \\
%         $k$ & Index to denote the $k$-th component of $\mathbf{F}$ & \\
%         $n$ & Index to denote the $n$-th initialisation of VA & \\
%         $q$ & Total number of functions in $\mathbfgl{\Theta}$ & \\
% \end{longtable}
% \end{center}

% \clearpage

% %%%%%%%%%%%%%%%%%%%%%%%%%%%%%%%%%%%%%%%%%%%%%%%%%%%%%%%%%%%%%%%%%%%%%
% \section{Cost function analysis}
% \label{SI-costfunk-analysis}

% Our aim is now to explore the landscape of the cost function as to understand the problem that we are solving and why it is very challenging. For illustrative purposes, in the following discussion we are only considering two dimensions of the cost function $\hat{A} = A_E+R_f A_M$.  We use the classical Lorenz system and take all parameters in the structure fixed and we add two extra parameters (highlighted in red),
% \begin{align}
%     \label{lorenzx2}
%     \dot{x} &= \sigma (y - x) + {\color{red}p_{1,1}},\\
%     \dot{y} &= x (\rho - z) - y + {\color{red}p_{2,1}},\\
%     \label{lorenzz2}
%     \dot{z} &= xy - \beta z.
% \end{align}

% We then vary these two parameters and plot what the cost function looks like, for three different values of $R_f$. The cost function that we want to minimise, is the one that has a large $R_f$ value (Figure \ref{figure_surfaces}, right).

% \begin{figure}[H]
%     \centering
%     \includegraphics[width=0.32\textwidth]{images/NMGP_Surface_p11_p21_Rf1_V2.png}
%     \includegraphics[width=0.32\textwidth]{images/NMGP_Surface_p11_p21_Rf2_V2.png}
%     \includegraphics[width=0.32\textwidth]{images/NMGP_Surface_p11_p21_Rf3_V2.png}
%     \caption{Varying $p_{1,1}$ and $p_{2,1}$ for three different $R_f$.}
%     \label{figure_surfaces}
% \end{figure}        

% The cost function $\hat{A}$ is highly non-convex and the task of finding its global minima a priori is a difficult task.

% % except for the parameter associated with the $y$ term in the equation for $y$ (highlighted in red), which will be our fee parameter.
% % \begin{align}
% %     \label{lorenzx}
% %     \dot{x} &= \sigma (y - x)\\
% %     \label{lorenzy}
% %     \dot{y} &= x (\rho - z) - {\color{red}y},\\
% %     \label{lorenzz}
% %     \dot{z} &= xy - \beta z.
% % \end{align}
% % We take that $\sigma = 10, \rho = 28, \beta = 8/3.$

% % In Figure \ref{figure_VA} (left) we show how equation $A_E+R_f A_M$ changes as we increase $R_f$ and as we vary our free parameter. We know that the minima of this function would be at when the varying parameter equals $-1$. We can observe that when $R_f = 0$ (blue) equation $\hat{A}$, although not completely smooth, has very few local minima. As we increase $R_f$ the smoothness decreases and more local minima appear in the function. For the largest $R_f$ value plotted (yellow) we see that the function is completely non-smooth and has a very large number of local minima. If one seeks the global minima of this function  when $R_f$ is large, which is the cost function one is seeking the minima for, the chances of ending up stuck in a local minima are large. 

% % \begin{figure}[htb!]
% %     \centering
% %     \includegraphics[width=0.45\textwidth]{images/Paper_Figure_VA.eps}
% %     %\hfill
% %     %\includegraphics[width=0.49\textwidth]{images/Paper_Figure_LASSO.eps}
% %     \caption{Left: Plot of $\hat{A}$ as we increase $R_f$ and as we vary the parameter that is associated with the $y$ term in equation \eqref{lorenzy}. Blue line corresponds to $R_f = 0$; red line corresponds to $R_f = 0.2147 \times 10^7$; green line corresponds to $0.6442 \times 10^7$; yellow line corresponds to $R_f = 1.0737 \times 10^7$. 
% %     %Right: Change of the argument of the $\min$ function in \eqref{lasso} as we vary the value of $\lambda$ and as we vary the parameter that is associated with the $y$ term in equation \eqref{lorenzy}.
% %     }
% %     \label{figure_VA}
% % \end{figure}

% % %Instead, with variational annealing method we start the search of this global minima in the blue curve ($R_f = 0$); the chances of finding the global minima in this curve increase considerably. Since the next iteration in the annealing process starts the search where the previous minima was found, we are likely to end up in the global minima as well when we have reached the yellow curve ($R_f = 1.0737 \times 10^7$). Still, multiple initialisations are needed to guarantee the discovery of the global minima.

% % % In Figure \ref{figure_VA_LASSO} (right) we show how the argument of the $\min$ function in \eqref{lasso} changes as we vary the value of $\lambda$ and as we vary the parameter that is associated with the $y$ term in equation \eqref{lorenzy}. We know that the minima of this function would be at when the varying parameter equals $-1$ when we set $\lambda = 0$. Blue line corresponds to $\lambda = 0$; red line corresponds to $\lambda = 100$; green line corresponds to $\lambda = 150$; yellow line corresponds to $\lambda = 200$. In this case we observe that the sparsity constraint term in \eqref{lasso}, as we increase $\lambda$, forces the minima of the function to be when the parameter associated with the $y$ term in equation \eqref{lorenzy} is $0$. In the context of model selection, this means that for a big enough $\lambda$ this term would not be picked up to describe the dynamics of our system. 

% % %In Figure \ref{figure_VA_LASSO_Together} we show how the equation $A = A_E+R_f A_M + \lambda \Vert \mathbf{p} \Vert_1$ changes as we increase $R_f$ and vary the value of $\lambda$, and as we vary the parameter that is associated with the $y$ term in equation \eqref{lorenzy}. We know that the minima of this function would be at when the varying parameter equals $-1$ when we set $\lambda = 0$.  
% % %In each sub-figure we can observe the variational annealing process at work, in which we are more likely to find the global minima by starting the minimisation at the $R_f = 0$ curves (blue) and then slowly increase $R_f$ until we end up finding the minima of the function of interest, that is, the function with $R_f = 1.0737 \times 10^7$.
% % %Now each sub-figure corresponds to a different $\lambda$ value. The result of increasing $\lambda$ is that for the first 3 subfigures (a), (b), (c), the parameter associated with the $y$ term in equation \eqref{lorenzy} is picked up in the model selected whereas for the last sub-figure (d) it is no longer picked up to describe the dynamics of our system.

% % % \begin{figure}[htb]
% % %     \centering
% % %     \includegraphics[width=\textwidth]{images/Paper_Figure_VA_LASSO.eps}
% % %     \caption{Plot of $A$ as we increase $R_f$ and vary the value of $\lambda$, and as we vary the parameter that is associated with the $y$ term in the $y$ equation for the classical Lorenz system. Blue lines correspond to $R_f = 0$; red lines correspond to $R_f = 0.2147 \times 10^7$; green lines correspond to $0.6442 \times 10^7$; yellow line correspond to $R_f = 1.0737 \times 10^7$. (a) $\lambda = 0$; (b) $\lambda = 175$; (c) $\lambda = 625$; (d) $\lambda = 2500$.}
% % %     \label{figure_VA_LASSO_Together}
% % % \end{figure}

% % % \clearpage
% % We now explore what happens if we add two extra terms in the original Lorenz system,
% % \begin{align}
% %     \label{lorenzx2}
% %     \dot{x} &= \sigma (y - x) + {\color{red}p_{1,1}},\\
% %     \dot{y} &= x (\rho - z) - y + {\color{red}p_{2,1}},\\
% %     \label{lorenzz2}
% %     \dot{z} &= xy - \beta z.
% % \end{align}

% % % \begin{figure}[htb!]
% % %     \centering
% % %     \includegraphics[width=0.32\textwidth]{images/NMGP_Surface_p11_p21_lambda1.png}
% % %     \includegraphics[width=0.32\textwidth]{images/NMGP_Surface_p11_p21_lambda2.png}
% % %     \includegraphics[width=0.32\textwidth]{images/NMGP_Surface_p11_p21_lambda3.png}
% % %     \caption{Varying $p_{1,1}$ and $p_{2,1}$ for three different $\lambda$ and $R_f = R_{f,\max}$ fixed.}
% % %     \label{figure_surfaces}
% % % \end{figure}    

% % \begin{figure}[htb!]
% %     \centering
% %     \includegraphics[width=0.32\textwidth]{images/NMGP_Surface_p11_p21_Rf1_V2.png}
% %     \includegraphics[width=0.32\textwidth]{images/NMGP_Surface_p11_p21_Rf2_V2.png}
% %     \includegraphics[width=0.32\textwidth]{images/NMGP_Surface_p11_p21_Rf3_V2.png}
% %     \caption{Varying $p_{1,1}$ and $p_{2,1}$ for three different $R_f$.}
% %     \label{figure_surfaces}
% % \end{figure}        

% % We have seen in this section that the cost function $\hat{A}$ is highly non-convex and that the task of finding its global minima a priori would be difficult.

% \clearpage

% %%%%%%%%%%%%%%%%%%%%%%%%%%%%%%%%%%%%%%%%%%%%%%%%%%%%%%%%%%%%%%%%%%%

% \section{AIC calculation for synthetic data}
% \label{SI-AICsynthetic}

% We want to find which model is the one that best represents the data synthetic data generated (in which we added some noise $\sim \mathcal{N}(0,0.01)$. Since we are working with chaotic systems, we only expect prediction up to the Lyapunov time of the system. The lowest Lyapunov time out of all the down-selected models for the synthetic data is $t_{M} \approx 1.2$. We use $S = 300$ time series of length $t_M$ as our validation set, but only consider the first 0.3 time units as to avoid further divergence. We also discard the first four points as they will be used to predict the initial condition for $y_0$ (\S \ref{SI-y0choice}). To calculate the AIC score, we define the residual sum of squares of the $m$-th model as
% \begin{equation}
%     \text{RSS}_m = \sum_{s=1}^S E^s_{av,m}(\mathbf{Y}_s,\mathbf{F}_m, \mathbf{p}_m),
% \end{equation}
% where $\mathbf{Y}_s=[x_e,z_e]_s$ is the synthetic data of the time-series $s$, $\mathbf{F}_m$ the governing equations of the $m$-th model, and $\mathbf{p}_m$ denotes the parameters found via parameter estimation for the $m$-th model. $E^s_{av,m}$ is the average absolute error over the time-series $s$ and is defined as
% \begin{equation}
%     \label{Eavm}
%     E^s_{av,m}(\mathbf{Y}_s,\mathbf{F}_m, \mathbf{p}_m) = \frac{1}{2M} \sum_{i=1}^M (x_{i,e}^s - x_i^s)^2 + (z_{i,e}^s - z_i^s)^2,
% \end{equation}
% where $x^s$ and $z^s$ denote the $x$ and $z$ component, respectively, of the solution of the $m$-th model in the $s$ time series, found via RK4 with $\Delta t = 0.01$.

% Finally, we can define the AIC of the $m$-th model as 
% \begin{equation}
%     \label{aic_def}
%     \text{AIC}_m = S \log \left( \frac{\sum_{s=1}^S E^s_{av,m}(\mathbf{Y}_s,\mathbf{F}_m, \mathbf{p}_m)}{S} \right) + 2N_{p,m}, %+ \frac{2(N_{p,m}+1)(N_{p,m}+2)}{S-N_{p,m}-2},
% \end{equation}
% where $N_{p,m}$ is the number of free parameters in the $m$-th model.

% We finally re-scale by the minimum AIC value, denoted by AIC$_{\text{min}}$, and so
% $\Delta \text{AIC}_m = \text{AIC}_m - \text{AIC}_{\text{min}}$. The only issue left to deal with before being able to compute the AIC for each model is how to calculate $x^s$ and $z^s$. 

% \subsection{$y_0$ choice}
% \label{SI-y0choice}

% We need an initial condition for each time series to be able to simulate each model. We have an initial condition for both $x$ and $z$ given by the experimental data, but we do not have any information for the $y$ component. 
% Let us consider the 8th order finite difference approximation of the time derivative of $x$
% \begin{equation}
%     \label{discretisation}
%     \frac{\ud x(t)}{\ud t} \approx \frac{
%       \splitfrac{
%         3x(t+4\Delta t)-32x(t+3\Delta t)+168x(t+2\Delta t)-672x(t+\Delta t)
%       }{
%         +672x(t+\Delta t)-168x(t+2\Delta t)+32x(t+3\Delta t)-3x(t+4\Delta t)
%       }
%       }{
%         840 \Delta t
%       }
% \end{equation}

% For each model, we have that 
% \begin{equation}
%     \label{eqforx_generic}
%     \frac{\ud x(t)}{\ud t} = F_{1,m}(x(t),y(t),z(t),\mathbf{p}_m).
% \end{equation}
% Putting equations \eqref{discretisation} and \eqref{eqforx_generic} together we have
% \begin{equation}
%     \label{approximation_xeq}
%     \frac{-x(t+2\Delta t) + 8x(t+\Delta t) - 8x(t-\Delta t) + x(t-2\Delta t)}{12 \Delta t} \approx F_{1,m}(x(t),y(t),z(t),\mathbf{p}_m).
% \end{equation}
% We need to solve for $y(0)$. We note that for the down-selected models in Section 2.1 in our manuscript the only terms with $y$ in the first equation in all the models is just the first order term, so for this case this is a particularly simple equation to solve.

% The results in the synthetic data indicate that there are only four candidate models that best represent the data. Even though the $\Delta$AIC from incorrect models (Figure \ref{figure_AIC_synthetic}, red, green and yellow lines) does not increase as we add more time series $S$ in the calculation of AIC, we consistently pick the correct model structure (blue line) as the one with lowest $\Delta AIC$.

% \begin{figure}[htb!]
%     \centering
%     \includegraphics[width=1\textwidth]{images/AIC_LorenzSynth_estimatedy0.png}
%     \caption{$\Delta$AIC from the different models DAHSI found using the synthetic data.}
%     \label{figure_AIC_synthetic}
% \end{figure}

% \clearpage

% \section{Down-selected models}
% \label{SI-downselected}

% We present the structure of the 25 down-selected models, but we do not provide the parameter estimation (the parameter values can be found in the code package).

% \begin{align}
% 	\frac{\ud x}{\ud t} &= p_{1,2}x+p_{1,3}y,\\
% 	\frac{\ud y}{\ud t} &= p_{2,2}x+p_{2,7}xz,\\
% 	\frac{\ud z}{\ud t} &= p_{3,4}z+p_{3,6}xy.
% \end{align}


% \begin{align}
% 	\frac{\ud x}{\ud t} &= p_{1,2}x+p_{1,3}y,\\
% 	\frac{\ud y}{\ud t} &= p_{2,2}x+p_{2,3}y+p_{2,7}xz,\\
% 	\frac{\ud z}{\ud t} &= p_{3,4}z+p_{3,6}xy.
% \end{align}


% \begin{align}
% 	\frac{\ud x}{\ud t} &= p_{1,2}x+p_{1,3}y+p_{1,4}z,\\
% 	\frac{\ud y}{\ud t} &= p_{2,2}x+p_{2,3}y+p_{2,7}xz,\\
% 	\frac{\ud z}{\ud t} &= p_{3,4}z+p_{3,6}xy.
% \end{align}


% \begin{align}
% 	\frac{\ud x}{\ud t} &= p_{1,1}+p_{1,2}x+p_{1,3}y,\\
% 	\frac{\ud y}{\ud t} &= p_{2,2}x+p_{2,7}xz,\\
% 	\frac{\ud z}{\ud t} &= p_{3,4}z+p_{3,6}xy.
% \end{align}


% \begin{align}
% 	\frac{\ud x}{\ud t} &= p_{1,1}+p_{1,2}x+p_{1,3}y+p_{1,4}z,\\
% 	\frac{\ud y}{\ud t} &= p_{2,2}x+p_{2,7}xz,\\
% 	\frac{\ud z}{\ud t} &= p_{3,4}z+p_{3,6}xy.
% \end{align}


% \begin{align}
% 	\frac{\ud x}{\ud t} &= p_{1,1}+p_{1,2}x+p_{1,3}y+p_{1,4}z,\\
% 	\frac{\ud y}{\ud t} &= p_{2,1}+p_{2,2}x+p_{2,3}y+p_{2,7}xz,\\
% 	\frac{\ud z}{\ud t} &= p_{3,4}z+p_{3,6}xy.
% \end{align}


% \begin{align}
% 	\frac{\ud x}{\ud t} &= p_{1,2}x+p_{1,3}y,\\
% 	\frac{\ud y}{\ud t} &= p_{2,2}x+p_{2,7}xz,\\
% 	\frac{\ud z}{\ud t} &= 0.
% \end{align}


% \begin{align}
% 	\frac{\ud x}{\ud t} &= p_{1,2}x+p_{1,3}y,\\
% 	\frac{\ud y}{\ud t} &= p_{2,2}x+p_{2,7}xz,\\
% 	\frac{\ud z}{\ud t} &= p_{3,6}xy.
% \end{align}


% \begin{align}
% 	\frac{\ud x}{\ud t} &= p_{1,2}x+p_{1,3}y,\\
% 	\frac{\ud y}{\ud t} &= p_{2,2}x+p_{2,3}y+p_{2,7}xz,\\
% 	\frac{\ud z}{\ud t} &= 0.
% \end{align}


% \begin{align}
% 	\frac{\ud x}{\ud t} &= p_{1,1}+p_{1,2}x+p_{1,3}y,\\
% 	\frac{\ud y}{\ud t} &= p_{2,2}x+p_{2,7}xz+,\\
% 	\frac{\ud z}{\ud t} &= 0.
% \end{align}


% \begin{align}
% 	\frac{\ud x}{\ud t} &= p_{1,2}x+p_{1,3}y,\\
% 	\frac{\ud y}{\ud t} &= p_{2,2}x+p_{2,3}y+p_{2,7}xz,\\
% 	\frac{\ud z}{\ud t} &= p_{3,6}xy.
% \end{align}


% \begin{align}
% 	\frac{\ud x}{\ud t} &= p_{1,2}x+p_{1,3}y+p_{1,4}z,\\
% 	\frac{\ud y}{\ud t} &= p_{2,2}x+p_{2,3}y+p_{2,7}xz,\\
% 	\frac{\ud z}{\ud t} &= 0.
% \end{align}


% \begin{align}
% 	\frac{\ud x}{\ud t} &= p_{1,1}+p_{1,2}x+p_{1,3}y,\\
% 	\frac{\ud y}{\ud t} &= p_{2,2}x+p_{2,7}xz,\\
% 	\frac{\ud z}{\ud t} &= p_{3,6}xy.
% \end{align}


% \begin{align}
% 	\frac{\ud x}{\ud t} &= p_{1,2}x+p_{1,3}y+p_{1,4}z,\\
% 	\frac{\ud y}{\ud t} &= p_{2,2}x+p_{2,7}xz,\\
% 	\frac{\ud z}{\ud t} &= p_{3,4}z+p_{3,6}xy.
% \end{align}


% \begin{align}
% 	\frac{\ud x}{\ud t} &= p_{1,2}x+p_{1,3}y+p_{1,4}z,\\
% 	\frac{\ud y}{\ud t} &= p_{2,2}x+p_{2,3}y+p_{2,7}xz,\\
% 	\frac{\ud z}{\ud t} &= p_{3,6}xy.
% \end{align}


% \begin{align}
% 	\frac{\ud x}{\ud t} &= p_{1,1}+p_{1,2}x+p_{1,3}y+p_{1,4}z,\\
% 	\frac{\ud y}{\ud t} &= p_{2,2}x+p_{2,7}xz,\\
% 	\frac{\ud z}{\ud t} &= p_{3,6}xy.
% \end{align}


% \begin{align}
% 	\frac{\ud x}{\ud t} &= p_{1,2}x+p_{1,3}y+p_{1,4}z,\\
% 	\frac{\ud y}{\ud t} &= p_{2,2}x+p_{2,7}xz,\\
% 	\frac{\ud z}{\ud t} &= p_{3,4}z+p_{3,6}xy+p_{3,7}xz.
% \end{align}


% \begin{align}
% 	\frac{\ud x}{\ud t} &= p_{1,1}+p_{1,2}x+p_{1,3}y+p_{1,4}z,\\
% 	\frac{\ud y}{\ud t} &= p_{2,2}x+p_{2,3}y+p_{2,7}xz,\\
% 	\frac{\ud z}{\ud t} &= p_{3,6}xy.
% \end{align}


% \begin{align}
% 	\frac{\ud x}{\ud t} &= p_{1,2}x+p_{1,3}y+p_{1,4}z,\\
% 	\frac{\ud y}{\ud t} &= p_{2,2}x+p_{2,6}xy+p_{2,7}xz,\\
% 	\frac{\ud z}{\ud t} &= p_{3,4}z+p_{3,6}xy+p_{3,7}xz.
% \end{align}


% \begin{align}
% 	\frac{\ud x}{\ud t} &= p_{1,1}+p_{1,2}x+p_{1,3}y+p_{1,4}z,\\
% 	\frac{\ud y}{\ud t} &= p_{2,2}x+p_{2,7}xz,\\
% 	\frac{\ud z}{\ud t} &= p_{3,4}z+p_{3,6}xy+p_{3,7}xz.
% \end{align}


% \begin{align}
% 	\frac{\ud x}{\ud t} &= p_{1,1}+p_{1,2}x+p_{1,3}y+p_{1,4}z,\\
% 	\frac{\ud y}{\ud t} &= p_{2,1}+p_{2,2}x+p_{2,3}y+p_{2,7}xz,\\
% 	\frac{\ud z}{\ud t} &= p_{3,6}xy.
% \end{align}


% \begin{align}
% 	\frac{\ud x}{\ud t} &= p_{1,2}x+p_{1,3}y+p_{1,4}z,\\
% 	\frac{\ud y}{\ud t} &= p_{2,2}x+p_{2,3}y+p_{2,6}xy+p_{2,7}xz,\\
% 	\frac{\ud z}{\ud t} &= p_{3,4}z+p_{3,6}xy+p_{3,7}xz.
% \end{align}


% \begin{align}
% 	\frac{\ud x}{\ud t} &= p_{1,1}+p_{1,2}x+p_{1,3}y+p_{1,4}z,\\
% 	\frac{\ud y}{\ud t} &= p_{2,2}x+p_{2,6}xy+p_{2,7}xz,\\
% 	\frac{\ud z}{\ud t} &= p_{3,4}z+p_{3,6}xy+p_{3,7}xz.
% \end{align}


% \begin{align}
% 	\frac{\ud x}{\ud t} &= p_{1,1}+p_{1,2}x+p_{1,3}y+p_{1,4}z,\\
% 	\frac{\ud y}{\ud t} &= p_{2,2}x+p_{2,3}y+p_{2,6}xy+p_{2,7}xz,\\
% 	\frac{\ud z}{\ud t} &= p_{3,4}z+p_{3,6}xy+p_{3,7}xz.
% \end{align}


% \begin{align}
% 	\frac{\ud x}{\ud t} &= p_{1,1}+p_{1,2}x+p_{1,3}y+p_{1,4}z,\\
% 	\frac{\ud y}{\ud t} &= p_{2,1}+p_{2,2}x+p_{2,3}y+p_{2,6}xy+p_{2,7}xz,\\
% 	\frac{\ud z}{\ud t} &= p_{3,4}z+p_{3,6}xy+p_{3,7}xz.
% \end{align}

% \subsection{Models identified in the Pareto front edge}
% \label{SI-Paretomodels}

% \begin{table}[H]
% \centering
% \caption{Models identified in the Pareto front in Figure 1(d) in the main manuscript.}
% \label{table_params_comparison_pareto}
%     \resizebox{0.78\textwidth}{!}{%
%     \begin{tabular}{l|r|rrrrrrr}
%      & & \multicolumn{7}{c}{number of active terms} \\
%      & Term & 6 & 7 & 8 & 9 & 10 & 11 & 12 \\ \hline
%     \multirow{10}{*}{eq. $\dot{x}$} & $1$ & 0 & 0 & -0.8112 & 0 & 0 & -0.2514 & -2.4053 \\
%     & $x$ & -16.5556 & -16.9554 & -16.4666 & -16.5603 & -17.0172 & -17.0582 & -17.0627 \\  
%     & $y$ & 19.8000 & 18.7853 & 19.8120 & 16.7514 & 19.9884 & 19.9840 & 19.9862 \\  
%     & $z$ & 0 & 0 & 0.0276 & 0.1486 & 0.1596 & 0.1833 & 1.4595 \\  
%     & $x^2$ & 0 & 0 & 0 & 0 & 0 & 0 & 0 \\  
%     & $xy$ & 0 & 0 & 0 & 0 & 0 & 0 & 0 \\  
%     & $xz$ & 0 & 0 & 0 & 0 & 0 & 0 & 0 \\  
%     & $y^2$ & 0 & 0 & 0 & 0 & 0 & 0 & 0 \\  
%     & $yz$ & 0 & 0 & 0 & 0 & 0 & 0 & 0 \\  
%     & $z^2$ & 0 & 0 & 0 & 0 & 0 & 0 & 0 \\  \hline
%     \multirow{10}{*}{eq. $\dot{y}$} & $1$ & 0 & 0 & 0 & 0 & 0 & 0 & 0.7892 \\
%     & $x$ & 23.2613 & 24.3535 & 23.0763 & 27.3789 & 22.6028 & 22.6017 & 22.6061 \\  
%     & $y$ & 0 & 0.2580 & 0 & 0 & 0.3346 & 0.3567 & 0.3298 \\  
%     & $z$ & 0 & 0 & 0 & 0 & 0 & 0 & 0 \\  
%     & $x^2$ & 0 & 0 & 0 & 0 & 0 & 0 & 0 \\  
%     & $xy$ & 0 & 0 & 0 & -0.0922 & -0.0906 & -0.0843 & -0.3647 \\  
%     & $xz$ & -6.3345 & -6.7054 & -6.2868 & -7.4621 & -6.2507 & -6.2561 & -6.2691 \\  
%     & $y^2$ & 0 & 0 & 0 & 0 & 0 & 0 & 0 \\  
%     & $yz$ & 0 & 0 & 0 & 0 & 0 & 0 & 0 \\  
%     & $z^2$ & 0 & 0 & 0 & 0 & 0 & 0 & 0 \\  \hline
%     \multirow{10}{*}{eq. $\dot{z}$} & $1$ & 0 & 0 & 0 & 0 & 0 & 0 & 0 \\
%     & $x$ & 0 & 0 & 0 & 0 & 0 & 0 & 0 \\  
%     & $y$ & 0 & 0 & 0 & 0 & 0 & 0 & 0 \\  
%     & $z$ & -3.6646 & -3.6835 & -3.6736 & 4.3951 & -3.6954 & -3.6966 &  -3.6941 \\  
%     & $x^2$ & 0 & 0 & 0 & 0 & 0 & 0 & 0 \\  
%     & $xy$ & 5.1948 & 4.8273 & 5.2315 & -3.6660 & 5.1412 & 5.1292 & 5.1326  \\  
%     & $xz$ & 0 & 0 & 0 & 0.0883 & 0.0903 & 0.0791 & 0.2900 \\  
%     & $y^2$ & 0 & 0 & 0 & 0 & 0 & 0 & 0 \\  
%     & $yz$ & 0 & 0 & 0 & 0 & 0 & 0 & 0 \\  
%     & $z^2$ & 0 & 0 & 0 & 0 & 0 & 0 & 0 \\  \hline    
%     RSS &  & 3.8233 & 3.6921 & 3.6574 & 3.6444 & 3.5672 & 3.5419 & 3.5579 \\ 
%     \end{tabular}
%     }      
% \end{table}   

% \subsection{AIC and BIC on the 25 down-selected models}
% \label{SI-aic-bic-experimental}
% Bayesian information criteria (BIC) is defined as 
% \begin{equation}
%     \text{BIC}_m = S \log \left( \frac{\sum_{s=1}^S E^s_{av,m}(\mathbf{Y}_s,\mathbf{F}_m, \mathbf{p}_m)}{S} \right) + S \log(N_{p,m}). %+ \frac{2(N_{p,m}+1)(N_{p,m}+2)}{S-N_{p,m}-2},
% \end{equation}
% In the same way as we did in \S \ref{SI-AICsynthetic}, we re-scale by the minimum BIC value, denoted by BIC$_{\text{min}}$, and so
% $\Delta \text{BIC}_m = \text{BIC}_m - \text{BIC}_{\text{min}}$.

% For both $\Delta \text{AIC}_m$ and $\Delta \text{BIC}_m$ we presented here we are able to consistently identify a unique model using Akaike information criteria and Bayesian information criteria (Figure \ref{figure_AIC_BIC_experimental}). If we just look at the Pareto front, one might ask if the decrease between 9 and 10 terms is meaningful. AIC says that it is.

% \begin{figure}[htb!]
%     \centering
%     \includegraphics[width=1\textwidth]{images/AIC_1080ish_randomsamples.png}
%     \includegraphics[width=1\textwidth]{images/BIC_1080ish_randomsamples.png}
%     \caption{$\Delta \text{AIC}_m$ and $\Delta \text{BIC}_m$ from the different models DAHSI found using the experimental data in \cite{Blakely2007}. For each $S$ in the x-axis, we pick $S$ random time samples.}
%     \label{figure_AIC_BIC_experimental}
% \end{figure}

% \clearpage

% %%%%%%%%%%%%%%%%%%%%%%%%%%%%%%%%%%%%%%%%%%%%%%%%%%%%%%%%%%%%%%%%%%%

% \section{Action derivation}
% \label{SI-action-derivation}

% Our goal is to find $\mathbf{X}$ and $\mathbf{p}$ that maximise the probability $P(\mathbf{X}, \mathbf{p} \; | \; \mathbf{Y}, \mathbf{\hat{F}})$. We have that \cite{Abarbanel2013}
% \begin{equation}
%     P(\mathbf{X}, \mathbf{p} \; | \; \mathbf{Y}, \mathbf{\hat{F}}) = \int \exp\left[ -A_0(\mathbf{X},\mathbf{Y}) \right] \; \ud \mathbf{X}.
% \end{equation}
% Furthermore,
% \begin{equation}
%     \label{action}
%     A_0(\mathbf{X},\mathbf{Y}) = - \sum_{i=1}^N \text{CMI}\left[\mathbf(t_i),\mathbf{Y}(t_i) \; | \; \mathbf{Y}(t_0),\dots,\mathbf{Y}(t_{i-1})\right] - \sum_{i=1}^{N-1} \log\left[ P(\mathbf{X}(t_{i+1}),\mathbf{p} \; | \; \mathbf{X}(t_{i}), \mathbf{\hat{F}}) \right],
% \end{equation}

% We make the following assumptions:
% \begin{enumerate}
%     \item The measurements $\mathbf{Y}$ have uncorrelated Gaussian error and that there is no correlation between errors in measuring different quantities or at varying time points \cite{Abarbanel2013};
%     \item The state at the next time point depends only on the state at the current time point, and that our model can have some error by widening the $\delta$ function it would follow otherwise using a Gaussian approximation of it \cite{Abarbanel2013};
%     \item Each element in $\mathbf{p}$ follows a Laplace distribution with \emph{mean} $0$ and diversity $b$.
% \end{enumerate}

% With assumption 1. it can be shown that \cite{Abarbanel2013}
% \begin{equation}
%     \text{CMI}\left[\mathbf(t_i),\mathbf{Y}(t_i) \; | \; \mathbf{Y}(t_0),\dots,\mathbf{Y}(t_{i-1})\right] = \frac{1}{2 \sigma_m^2} \sum_{l=1}^L \left(x_l(t_i) - y_l(t_i)\right)^2
% \end{equation}

% For the second term in the sum, we need to find an expression for $P(\mathbf{X}(t_{i+1}),\mathbf{p} \; | \; \mathbf{X}(t_{i}), \mathbf{\hat{F}})$. Let us now focus on the $k$-th component of $\mathbf{X}(t_{i+1})$, and so our goal is to find an expression for $P(x_k(t_{i+1}), \mathbf{p}_k \; | \; \mathbf{X}(t_{i}), F_k)$. 

% We consider the library of $q$ possible functions and the generic expression for each equation of our model as in equation (8) in the main text. We can rewrite the probability we are seeking as
% \begin{equation}
%     \label{main_eq_action}
%     P(x_k(t_{i+1}),\mathbf{p}_k \; | \; \mathbf{X}(t_i), F_k) = P(\mathbf{p}_k \; | \; x_k(t_{i+1}), \mathbf{X}(t_i), F_k) P(x_k(t_{i+1}) \; | \; \mathbf{X}(t_i), F_k).
% \end{equation}
% Now each term in the right hand side can also be rewritten as
% \begin{align}
%     P(\mathbf{p}_k \; | \; x_k(t_{i+1}), \mathbf{X}(t_i), F_k) &= \frac{P(x_k(t_{i+1}),\mathbf{X}(t_i), F_k \; | \; \mathbf{p}_k) P(\mathbf{p}_k)}{P(x_k(t_{i+1}),\mathbf{X}(t_i), F_k)}, \\
%     P(x_k(t_{i+1}) \; | \; \mathbf{X}(t_i), F_k) &= \frac{P(x_k(t_{i+1}),\mathbf{X}(t_i), F_k)}{P(\mathbf{X}(t_i),F_k)}.    
% \end{align}

% Thus, equation \eqref{main_eq_action} becomes
% \begin{equation}
%     \label{main_eq_action_2}
%     P(x_k(t_{i+1}),\mathbf{p}_k \; | \; \mathbf{X}(t_i), F_k) = \frac{P(x_k(t_{i+1}),\mathbf{X}(t_i), F_k \; | \; \mathbf{p}_k) P(\mathbf{p}_k)}{P(\mathbf{X}(t_i),F_k)}.
% \end{equation}

% We can rewrite the first therm on the right hand side in equation \eqref{main_eq_action_2} as a likelihood,
% \begin{equation}
%     P(x_k(t_{i+1}),\mathbf{X}(t_i), F_k \; | \; \mathbf{p}_k) = \mathcal{L}(\mathbf{p}_k \; | \; x_k(t_{i+1}),\mathbf{X}(t_i), F_k).
% \end{equation}
% Assuming that our next state follows a normal distribution with mean $f_k$ and standard deviation $\sigma^2$,
% \begin{equation}
%     \mathcal{L}(\mathbf{p}_k \; | \; x_k(t_{i+1}),\mathbf{X}(t_i), F_k) = \frac{1}{\sigma \sqrt{2\pi}} \exp{
%     \left(
%     -\frac{
%     \left[ 
%     x_k(t_{i+1}) - f_k(\mathbf{X},\mathbf{p},F_k) \right]^2
%     }{2\sigma^2}
%     \right)
%     }.
% \end{equation}
% With assumption 3., we know that each $p_{k,j}$ follows a Laplace distribution,
% \begin{equation}
%     p_{k,j} \sim \text{Laplace}(0,b) = \frac{1}{2b}\exp{\left(-\frac{|p_{k,j}|}{b}\right)},
% \end{equation}
% and so
% \begin{equation}
%     P(\mathbf{p}_k) = \prod_{j=1}^q \frac{1}{2b}\exp{\left(-\frac{|p_{k,j}|}{b}\right)}.
% \end{equation}

% With this we can write equation \eqref{main_eq_action_2} as
% \begin{equation}
%     \begin{split}
%     \label{main_eq_action_3}
%         P(&x_k(t_{i+1}),\mathbf{p}_k \; | \; \mathbf{X}(t_i), F_k) \propto \\
%         &\propto \frac{1}{\sigma \sqrt{2\pi}} \exp{\left(-\frac{\left[ x_k(t_{i+1}) - f_k(\mathbf{X},\mathbf{p},F_k) \right]^2}{2\sigma^2}\right)} \prod_{j=1}^q \frac{1}{2b}\exp{\left(-\frac{|p_{k,j}|}{b}\right)}.        
%     \end{split}
% \end{equation}
% Note that since we are going to be minimising the action $A_0$ (equaton \eqref{action}) we forget about the constant term $P(\mathbf{X}(t_i), F_k)$ in the denominator and we are good with just having this proportionality instead of an equality.

% Note that because the $k$-th current state only depends upon the previous one,
% \begin{equation}
%     P\left(\mathbf{X}(t_{i+1}), \mathbf{p} \; | \; \mathbf{X}(t_{i}), \mathbf{\hat{F}}\right) = \prod_{k=1}^D P(x_k(t_{i+1}), \mathbf{p}_k \; | \; \mathbf{X}(t_i), F_k),
% \end{equation}
% and so, finally, we can write
% \begin{equation}
%     \begin{split}
%     \label{main_eq_action_4}
%         P(&\mathbf{X}(t_{i+1}),\mathbf{p} \; | \; \mathbf{X}(t_{i}), \mathbf{\hat{F}}) \propto \\ &\propto \prod_{k=1}^D \left\{ \frac{1}{\sigma \sqrt{2\pi}} \exp{\left(-\frac{\left[ x_k(t_{i+1}) - f_k(\mathbf{X},\mathbf{p},F_k) \right]^2}{2\sigma^2}\right)} \prod_{j=1}^q \frac{1}{2b}\exp{\left(-\frac{|p_{k,j}|}{b}\right)}\right\}.
%     \end{split}
% \end{equation}

% Upon taking the logarithm to this expression above,
% \begin{equation}
%     \label{main_eq_action_5}
%         \log(P(\mathbf{X}(t_{i+1}),\mathbf{p} \; | \; \mathbf{X}(t_{i}), \mathbf{\hat{F}})) \propto \sum_{k=1}^D \left\{ -\frac{\left[ x_k(t_{i+1}) - f_k(\mathbf{X},\mathbf{p},F_k) \right]^2}{2\sigma^2} - \lambda \Vert \mathbf{p}_k \Vert_1 \right\} + \frac{D}{\sigma \sqrt{2\pi}} + \frac{\lambda D}{2},
% \end{equation}
% where $\lambda = q/b$. %Since $\frac{D}{\sigma \sqrt{2\pi}} + \frac{\lambda D}{2}$ something, we can just use the first term in equation \eqref{main_eq_action_5}. 

% We have seen that equation \eqref{action} becomes
% \begin{equation}
%     \label{costfunk-appendix}
%     A(\mathbf{X},\mathbf{p}) = \frac{1}{N}\sum_{i=1}^N \Vert \mathbf{X}(t_{i}) - \mathbf{Y}(t_{i}) \Vert^2 + \frac{1}{N}\sum_{i=1}^{N-1} R_f \left\{ \Vert \mathbf{X}(t_{i+1}) - \mathbf{f}(\mathbf{X}(t_n),\mathbf{p},\mathbf{\hat{F}}) \Vert^2 \right\} + \lambda \Vert \mathbf{p} \Vert_1,
% \end{equation}
% which is what we wanted to show.

% \clearpage

% %%%%%%%%%%%%%%%%%%%%%%%%%%%%%%%%%%%%%%%%%%%%%%%%%%%%%%%%%%%%%%%%%%%

% \section{Computational time}
% \label{SI-computationaltime}

% We use the Lorenz system, with all variables observed, $N=1001$ time points, $\Delta t = 0.01$, and no noise. The more terms our library $\mathbfgl{\Theta}$, the more time it takes to evaluate the cost function associated, its Jacobian and its Hessian (Figure \ref{figure_computational}(left)).
% However, due to model symmetries and other structural features, the time to run our algorithm does not monotonically increase with increasing number of terms in our library. A library with 10 terms can take 100 times more to run than the full library of monomials up to degree two in three variables (Figure \ref{figure_computational}(right)).

% \begin{figure}[htb!]
%     \centering
%     \includegraphics[width=0.49\textwidth]{images/terms_vs_callIPOPT.pdf}
%     \includegraphics[width=0.49\textwidth]{images/terms_vs_timerun.pdf}
%     \caption{7 terms: parameter estimation. 10 terms: in blue $x^2$ in each equation; in red $1$ in each equation. 13 terms: $x^2$ and $y^2$ in each equation. 16 terms: $x^2$, $y^2$ and $z^2$ in each equation. 19 terms: $1$, $x^2$, $y^2$ and $z^2$ in each equation. 30 terms: model selection.}
%     \label{figure_computational}
% \end{figure}

% \clearpage

% %%%%%%%%%%%%%%%%%%%%%%%%%%%%%%%%%%%%%%%%%%%%%%%%%%%%%%%%%%%%%%%%%%%%%

% \section{Semiconductor}
% \label{SI-semiconductor}

% We consider this semiconductor model ($T$ trap levels with two possible states differing by one electronic unit
% of charge),
% \begin{align}
%     \label{eq-n}
%     \frac{\ud x}{\ud t} &= e_{n,01} y - R_{n,10} xz,\\
%     \frac{\ud y}{\ud t} &= -e_{n,01} y + R_{n,10} xz,\\
%     \label{eq-nd1}
%     \frac{\ud z}{\ud t} &= e_{n,01} y - R_{n,10} xz. 
% \end{align}
% $x$ denotes the number of electrons in the conduction band, $y$ denotes the number of traps with 2 electrons, and $z$ denotes the number of traps with 1 electron. We chose $e_{n,01} = 0.5$ and $R_{n,10} = 0.25$.

% \begin{figure}[H]
%     \centering
%     \includegraphics[width=.45\textwidth]{images/time_series_semicond.pdf}
%     \caption{Dynamics from the original system \eqref{eq-n}-\eqref{eq-nd1}.}
%     \label{figure_SemiCond_timeseries}
% \end{figure}

% Instead of using the library of all monomials in three variables up to degree two, we know that there are only a few terms make sense physically \cite{}. Our generic model for this example is
% \begin{align}
%     \frac{\ud x}{\ud t} &= p_{1,1} + p_{1,2} x + p_{1,3} y + p_{1,4} z + p_{1,5} x^2 + p_{1,7} xz,\\
%     \frac{\ud y}{\ud t} &= p_{2,1} + p_{2,2} x + p_{2,3} y + p_{2,4} z + p_{2,5} x^2 + p_{2,7} xz,\\
%     \frac{\ud z}{\ud t} &= p_{3,1} + p_{3,2} x + p_{3,3} y + p_{3,4} z + p_{3,7} xz.   
% \end{align}

% We first consider three observed variables, $D=L=3$. 
% We consider a time series of $N = 101$ equally spaced time points, with $\Delta t = 0.01$. The $\lambda$ sweep results in a different amount of active terms for each value. See Figure \ref{figure_lambdasweep_semicond} (left). Since we know the model from which our data comes from, we just want to see if the model that has the right number of terms (highlighted in red) corresponds to our original one. This corresponds to $\lambda \in [0.0, 0.0]$ and it has indeed the right sparsity pattern.

% \subsection{1 hidden variable}

% We consider two observed variables, $L=2$. We pick $x$ and $y$. We run $N_I = 1000$ different initialisations. There is a question in this particular case on how the initial guess should be picked that we will discuss in a later section.
% We do a $\lambda$ sweep from $\lambda = 0.1$ through $\lambda = 0.3$. Out of all the 1,000 different initialisations, we recover the right sparsity pattern 68 times. The optimal $\lambda = 0.19$, for which we recover the right sparsity pattern 33 times (see Figure \ref{figure_lambdasweep_Grad}).

% \begin{table}[H]
%     \centering
%     %\resizebox{\textwidth}{!}{%
%     \begin{tabular}{ccccccc}
%     \hline
%     observed & hidden & N & $\Delta$ t & $\beta_{\max}$ & $\lambda$ & recovery \\ \specialrule{1.3pt}{1pt}{1pt}
%     2 & 1 ($z$) & 101 & 0.01 & 30 & 0.19 & 3.3\% \\ \hline
%     \end{tabular}%}
%     \caption{}
% \end{table}

% \begin{figure}[H]
%     \centering
%     \includegraphics[width=0.45\textwidth]{images/lambda_sweep_allobserved.pdf}
%     \hspace{10mm}
%     \includegraphics[width=0.45\textwidth]{images/lambda_sweep_1hidden.pdf}
%     \caption{Left: all observed variables. Right: one hidden variable. Highlighted in red are the $\lambda$ that lead to model recovery.}
%     \label{figure_lambdasweep_semicond}
% \end{figure}  

% \begin{figure}[htb!]
%     \centering
%     \includegraphics[width=0.45\textwidth]{images/recovery_rate_sweep_Grad.pdf}
%     \caption{Percentage of recovery rate for different $\lambda$ values for 1,000 different initialisations. Initial guess for unmeasured variables is obtained through the derivatives of the measured variables.}
%     \label{figure_lambdasweep_Grad}
% \end{figure}

% \subsection{Initial guess}

% \begin{algorithm}
% \caption{Algorithm for picking an initial guess for unobserved variables}
% \label{Algorithm_IniGuess}    
%     \begin{algorithmic}[1]
    
%     % \Procedure{}{}
%         \For{$d = 1:(D-L)$}   \Comment{loop in unmeasured variables}
        
%             \State Pick at random one of the observed variables.
            
%             \State $dX_d \leftarrow$ Calculate gradient vector from its time series.
            
%             \While{$Z_d$ out of bounds} \Comment{Make sure unmeasured variable is within bounds}  
%                 \State $Z_d(t_1) \leftarrow$ Random initial condition for unobserved variable within bounds.
                
%                 \For{$i = 1:N-1$} 
%                     \State $Z_d(t_{i+1}) = \Delta t \times dX_d(t_i) + Z_d(t_i)$ 
%                 \EndFor
%             \EndWhile
%         \EndFor            
%     % \EndProcedure

%     \end{algorithmic}
% \end{algorithm}

% \subsection{Parameter identifiability}
% \label{SI-parameter-identif}

% There are two main reasons of why a parameter might not be identifiable: said parameter does not influence the model output; there is a interdependence among different parameters, that is, one can compensate the change of one parameter (that would influence the model output) by changing other parameter(s) and have the output be the same. In this section, we focus on the latter.

% One way to detect pairwise interplay is by plotting contours of the cost function versus pairs of parameters. Largely eccentric contours or \emph{valleys} show that the cost function is almost unchanged in one direction, and the two parameters are highly correlated. 
% The main drawback for our case in particular is that we will be limited to find relationships only between pairs of parameters instead of higher dimensional interactions. In \cite{Gabor2017} they present how to find these higher dimensional interactions by a measure named \emph{the collinearity of parametric sensitivities}.

% Consider the generic model (except that the right terms are fixed -- highlighted in blue; $e_{n,01} = 0.5$, $R_{n,10} = 0.25$)
% \begin{align}
%     \frac{\ud x}{\ud t} &= p_{1,1} + p_{1,2} x \textcolor{blue}{\,+\,e_{n,01}} y + p_{1,4} z + p_{1,5} x^2 \textcolor{blue}{\,-\,R_{n,10}} xz,\\
%     \frac{\ud y}{\ud t} &= p_{2,1} + p_{2,2} x \textcolor{blue}{\,-\,e_{n,01}} y + p_{2,4} z + p_{2,5} x^2 \textcolor{blue}{\,+\,R_{n,10}} xz,\\
%     \frac{\ud z}{\ud t} &= p_{3,1} + p_{3,2} x \textcolor{blue}{\,+\,e_{n,01}} y + p_{3,4} z \textcolor{blue}{\,-\,R_{n,10}} xz.   
% \end{align}
% We will now add only two extra parameters (two of the black terms) at a time. Each Figure \ref{figure_identi_1}-\ref{figure_identi_4} is obtained by picking one term (parameter 1, which is the first extra term in the system), and then study the cost function by adding another term (parameter 2, which is the second extra term in the system). We study this for all the possibles ``parameter 2''.

% Take Figure \ref{figure_identi_1}. Parameter 1 here is the term $1$ in the equation $\ud x / \ud t$. That is, $p_{1,1}$. This extra term is fixed for all subplots. Then parameter 2 (the second extra term) corresponds to (in order of subplots) $p_{1,2}, \, p_{1,4}, \, p_{1,5}, \, p_{2,1}, \, p_{2,2}, \, p_{2,4}, \, p_{2,5}, \, p_{3,1}, \, p_{3,2} \, p_{3,4}$.

% Figures \ref{figure_identi_2}-\ref{figure_identi_4} follow the same logic. I have just done four figures because they already show identifiability problems.

% \begin{figure}
%     \centering
%     \includegraphics[height=0.195\textheight]{images/term1_2_1.png}
%     \includegraphics[height=0.195\textheight]{images/term1_2_2.png}\\
%     \includegraphics[height=0.195\textheight]{images/term1_2_3.png}
%     \includegraphics[height=0.195\textheight]{images/term1_2_4.png}\\
%     \includegraphics[height=0.195\textheight]{images/term1_2_5.png}
%     \includegraphics[height=0.195\textheight]{images/term1_2_6.png}\\
%     \includegraphics[height=0.195\textheight]{images/term1_2_7.png}
%     \includegraphics[height=0.195\textheight]{images/term1_2_8.png}\\
%     \includegraphics[height=0.195\textheight]{images/term1_2_9.png}
%     \includegraphics[height=0.195\textheight]{images/term1_2_10.png}
%     \caption{parameter 1 is $1$ on the $\ud x/\ud t$ equation.}
%     \label{figure_identi_1}
% \end{figure}

% \begin{figure}
%     \centering
%     \includegraphics[height=0.195\textheight]{images/term1_4_1.png}
%     \includegraphics[height=0.195\textheight]{images/term1_4_2.png}\\
%     \includegraphics[height=0.195\textheight]{images/term1_4_3.png}
%     \includegraphics[height=0.195\textheight]{images/term1_4_4.png}\\
%     \includegraphics[height=0.195\textheight]{images/term1_4_5.png}
%     \includegraphics[height=0.195\textheight]{images/term1_4_6.png}\\
%     \includegraphics[height=0.195\textheight]{images/term1_4_7.png}
%     \includegraphics[height=0.195\textheight]{images/term1_4_8.png}\\
%     \includegraphics[height=0.195\textheight]{images/term1_4_9.png}
%     \includegraphics[height=0.195\textheight]{images/term1_4_10.png}
%     \caption{parameter 1 is $x$ on the $\ud x/\ud t$ equation.}
%     \label{figure_identi_2}
% \end{figure}

% \begin{figure}
%     \centering
%     \includegraphics[height=0.195\textheight]{images/term1_3_1.png}
%     \includegraphics[height=0.195\textheight]{images/term1_3_2.png}\\
%     \includegraphics[height=0.195\textheight]{images/term1_3_3.png}
%     \includegraphics[height=0.195\textheight]{images/term1_3_4.png}\\
%     \includegraphics[height=0.195\textheight]{images/term1_3_5.png}
%     \includegraphics[height=0.195\textheight]{images/term1_3_6.png}\\
%     \includegraphics[height=0.195\textheight]{images/term1_3_7.png}
%     \includegraphics[height=0.195\textheight]{images/term1_3_8.png}\\
%     \includegraphics[height=0.195\textheight]{images/term1_3_9.png}
%     \includegraphics[height=0.195\textheight]{images/term1_3_10.png}
%     \caption{parameter 1 is $1$ on the $\ud y/\ud t$ equation.}
%     \label{figure_identi_3}
% \end{figure}

% \begin{figure}
%     \centering
%     \includegraphics[height=0.195\textheight]{images/term1_1_1.png}
%     \includegraphics[height=0.195\textheight]{images/term1_1_2.png}\\
%     \includegraphics[height=0.195\textheight]{images/term1_1_3.png}
%     \includegraphics[height=0.195\textheight]{images/term1_1_4.png}\\
%     \includegraphics[height=0.195\textheight]{images/term1_1_5.png}
%     \includegraphics[height=0.195\textheight]{images/term1_1_6.png}\\
%     \includegraphics[height=0.195\textheight]{images/term1_1_7.png}
%     \includegraphics[height=0.195\textheight]{images/term1_1_8.png}\\
%     \includegraphics[height=0.195\textheight]{images/term1_1_9.png}
%     \includegraphics[height=0.195\textheight]{images/term1_1_10.png}
%     \caption{parameter 1 is $z$ on the $\ud z/\ud t$ equation.}
%     \label{figure_identi_4}
% \end{figure}

% \clearpage 

% %%%%%%%%%%%%%%%%%%%%%%%%%%%%%%%%%%%%%%%%%%%%%%%%%%%%%%%%%%%%%%%%%%%%%

% \section{Predator-Prey}
% \label{SI-predtorprey}

% Although it is not very common to find \emph{pure} predator-prey interactions in nature, there is a classical set of data by the Hudson Bay company which corresponds the number of snowshoe hares and Canadian lynxes trapped in Canada, which in turn shows the relative population of both \cite{Odum1971, HareLynxWeb}. The data is recorded yearly, so $\Delta t = 1$. We use data between 1900 and 1920, thus $N = 21$. In this particular case we really do not know the dynamics behind the system although we know that the snowshoe hare is the primary food of the lynx. Therefore, we can assume that we have a predator-prey system, and there is the classical Lotka-Volterra model to describe these type of dynamics. We consider $L = D = 2$ (Figure \ref{figure_PredatorPrey}(a)). 
% We build the library of functions with all the monomials up to degree two in two variables, and with it we construct our generic model (Figure \ref{figure_PredatorPrey}(b)). We run our algorithm and varying $\lambda$ we obtain a list of possible models. By looking at the corresponding AIC values for each one, we find that the model with 7 active terms is the best one (Figure \ref{figure_PredatorPrey}(d)). We now consider that our generic model is the resulting model with 7 active terms. Again, we run the algorithm to find that the best model is one containing only 5 terms (Figure \ref{figure_PredatorPrey}(f-h)). We iterate this process, and run the algorithm considering the model with 5 active terms as the generic one. We find that the best model is the one containing 4 terms (Figure \ref{figure_PredatorPrey}(i-k)). This identified model corresponds to the Lotka-Volterra one. Once we do only parameter estimation on it, we obtain the dynamical system shown in Figure \ref{figure_PredatorPrey}(k). We compare the original data (dashed) with the resulting model (solid), which show an excellent match.

% \begin{figure}[htb]
%     \centering
%     \includegraphics[width=.85\textwidth]{images/Paper_Figure_PredatorPrey.pdf}
%     \caption{}
%     \label{figure_PredatorPrey}
% \end{figure}

% \clearpage

% %%%%%%%%%%%%%%%%%%%%%%%%%%%%%%%%%%%%%%%%%%%%%%%%%%%%%%%%%%%%%%%%%%%%%

% \section{$\alpha$ parameter in VA algorithm}

% We study how the parameter $\alpha$ used to increase the value of $R_f = R_{f,0} \alpha^{\beta}$ during the VA algorithm affects the recovery. We use the class Lorenz system,
% \begin{align}
%     \frac{\ud x}{\ud t} &= \sigma(y-x),\\
%     \frac{\ud y}{\ud t} &= x(\rho-z) - y,\\
%     \frac{\ud z}{\ud t} &= -\beta z + xy,
% \end{align}
% where $\sigma = 10$, $\rho = 28$, and $\beta = 8/3$. We numerically simulate the system using Runge-Kutta 4th order and a time step of $\Delta t = 0.01$, producing time-series similar to the experimental data set. 
% We add some error modeled as additive Gaussian noise of mean zero and standard deviation $\omega=0.01$. Therefore, the measurement function is $\mathbf{h}(\mathbf{X}) = \mathbf{X} + \mathcal{N}(0,\omega)$
% We consider $N=501$, and $y$ to be the hidden variable.

% As we increase $\alpha$ the recovery rate decreases, and for $\alpha \geq 1.3$ the recovery is 0\% (Table \ref{table_alpha}).

% \begin{table}[H]
% \centering
% \caption{Recovery rates for varying $\alpha$.}
% \label{table_alpha}
%     % \resizebox{0.98\textwidth}{!}{%
%     \begin{tabular}{cc}
%     $\alpha$ & recovery rate (\%) \\
%     \hline
%     1.1 & 93 \\ \hline
%     1.2 & 87 \\ \hline
%     1.25 & 20 \\ \hline
%     1.3 & 0 \\ \hline
%     1.4 & 0 \\ \hline
%     1.5 & 0  
%     \end{tabular}
%     % }
% \end{table} 

% \clearpage

% %%%%%%%%%%%%%%%%%%%%%%%%%%%%%%%%%%%%%%%%%%%%%%%%%%%%%%%%%%%%%%%%%%%%%

% \bibliography{bibliography_SI} 
% \bibliographystyle{siam}

% %%%%%%%%%%%%%%%%%%%%

% \end{document}
